# Supplementary material for: Network Memory Footprint Compression Through Jointly Learnable Codebooks and Mappings
Source: arXiv:2309.17361 source file (2023-09-29)
Supplement: Supplementary file 1 [file sota_mobnet_effnet.tex]

\begin{table*}[!t]
\caption{}
\label{tab:sota_mobilenet_efficientnet}
\centering
    \begin{tabular}{c|c|c|c|c|c}
     \hline
     architecture & method & Comp rate ($\alpha$) & optimization & integer & acc \\
     \hline
     \hline
     \multirow{9}{*}{MobileNet v2} & DFQ & 5.33 (W3/A16) & \xmark & \cmark & \\
                                & SQuant & 5.33 (W3/A16) & \xmark & \cmark & \\
                                & PowerQuant & 5.33 (W3/A16) & \xmark & \xmark & \\
                                & RED++ & 5.33 & \xmark & \xmark & \\
                                & FALL (init) & 7.5 & \xmark & \xmark & \\
                                \cline{2-5}
                                & AdaRound & 5.33 (W3/A16) & \cmark & \cmark & \\
                                & BrecQ & 5.33 (W3/A16) & \cmark & \cmark & \\
                                & NUPES & 5.33 (W3/A16) & \cmark & \xmark & \\
                                & FALL & 7.5 & \cmark & \xmark & \\
     \hline
     \multirow{9}{*}{EfficientNet B0}   & DFQ & 5.33 (W3/A16) & \xmark & \cmark & \\
                                & SQuant & 5.33 (W3/A16) & \xmark & \cmark & \\
                                & PowerQuant & 5.33 (W3/A16) & \xmark & \xmark & \\
                                & RED++ & 5.33 & \xmark & \xmark & \\
                                & FALL (init) & 7.5 & \xmark & \xmark & \\
                                \cline{2-5}
                                & AdaRound & 5.33 (W3/A16) & \cmark & \cmark & \\
                                & BrecQ & 5.33 (W3/A16) & \cmark & \cmark & \\
                                & NUPES & 5.33 (W3/A16) & \cmark & \xmark & \\
                                & FALL & 7.5 & \cmark & \xmark & \\
     \hline
    \end{tabular}
\end{table*}
